# Supplementary material for: Understanding three-body contributions to coarse-grained force-fields
Source: arXiv:1710.02188 source file (2017-10-05)
Supplement: Supplementary file 1 [file supporting_information.pdf]

# Supporting information

## Understanding three-body contributions to coarse-grained force-fields

Christoph Scherer[1, a)] and Denis Andrienko[1, b)]
*Max Planck Institute for Polymer Research, Ackermannweg 10, 55128 Mainz, Germany*

(Dated: 5 October 2017)

### I. SIMULATION DETAILS

All-atom simulations of liquid water are performed using the SPC/E water model.[1] For liquid methanol we employ the OPLS-AA force field[2,3] without constraints. In both cases, we use exactly the same parameter sets as in Ref. 4. We run atomistic simulations with the GROMACS package[5] (version 5.1). We equilibrate simulation boxes of 1000 molecules for 10 ns at 300 K and pressure of 1.0 bar using a stochastic dynamics algorithm[6] in combination with a Berendsen barostat[7] with a time constant of 1 ps, the compressibility parameter of water ($4.5 \cdot 10^{-5}\ ^1/_{\text{bar}}$), and a time step of 1 fs. Electrostatic interactions are treated with a particle mesh Ewald method[8] with cubic interpolation, a grid spacing of 0.12 nm and an Ewald accuracy of $1.0 \cdot 10^{-5}$. All short-ranged interactions (Van der Waals interactions and the short-range Coulomb part) are cut off at 1.2 nm and long-range dispersion corrections for energy and pressure are used. The equilibration runs are followed by 10 ns NVT production runs, again, using a stochastic dynamics algorithm, at the average density of the preceding NPT simulations, namely $\rho = 0.998\ ^{\text{g}}/_{\text{cm}^3}$ (water) and $\rho = 0.776\ ^{\text{g}}/_{\text{cm}^3}$ (methanol). These values are very close to the experimental densities at normal conditions ($p_{\text{ext}} = 1\,\text{atm}$, $T = 298\,\text{K}$): $\rho = 0.9971\ ^{\text{g}}/_{\text{cm}^3}$ (water)[9] and $\rho = 0.7872\ ^{\text{g}}/_{\text{cm}^3}$ (methanol).[10]

We conduct all CG simulations in the NVT ensemble at 300 K at the atomistic density using a system size of 1000 CG beads (representing 1000 molecules). For all CG simulations, we use the LAMMPS simulation package.[11] All two-body CG interactions are treated as tables using linear interpolation tables (LAMMPS pair_style table linear). In the case of three-body interactions, we extended the Sillinger-Weber interaction potential (LAMMPS pair_style sw) to read in tabulated angular dependent potentials (LAMMPS pair_style sw/table). We employ a chain of three Nose-Hoover thermostats[12,13] with a damping parameter of 200 fs integrating the equations of motion according to Ref. 14. In each case, we conduct 10 ns long production runs with a time step of 1 fs. All pair interactions are short-ranged and cut off at 1.2 nm.

### II. COARSE-GRAINING (CG)

As stated in the main text, we use single bead CG representations of atomistic water and methanol. In each case, we employ a center of mass mapping

$$\boldsymbol{R}_i = \sum_{\alpha \in i} w_\alpha \, \boldsymbol{r}_\alpha \,, \tag{II.1}$$

where $w_\alpha$ are the normalized masses ($w_\alpha = {}^{m_\alpha}/_{(\sum_{\alpha \in i} m_\alpha)}$) of each atom of molecule $i$. In this case, the mass of the CG bead is simply the sum of the atomistic masses, namely $M_i = 18.0154\,\text{amu}$ (water) and $M_i = 32.0374\,\text{amu}$ (methanol).

#### A. Iterative Boltzmann inversion (IBI)

To obtain the reference Iterative Boltzmann Inversion (IBI) potentials, we follow the description in Ref. 4. The initial guess of the CG potential is obtained via simple Boltzmann inversion: $U(r) = -k_{\text{B}} T \ln g(r)$ where $g(r)$ is the

a)Electronic mail: scherer@mpip-mainz.mpg.de
b)Electronic mail: denis.andrienko@mpip-mainz.mpg.de

radial distribution function. Then, the CG potential is iteratively refined, according to the following update scheme:

$$U^{(n+1)} = U^{(n)} + \alpha \Delta U^{(n)}, \tag{II.2}$$

$$\Delta U^{(n)} = k_{\mathrm{B}} T \ln \frac{g^{(n)}(r)}{g_{\mathrm{ref}}(r)}. \tag{II.3}$$

This empirical scheme reaches convergence as soon as the actual (radial) distribution function $g^{(n)}(r)$ matches the reference (radial) distribution function $g_{\mathrm{ref}}(r)$. We choose $\alpha = 1$, perform a simple smoothing of the potential at each iteration step and do not use any pressure correction. We stop the iterations after $N = 300$ steps. At this point, the potential has fully converged within the accuracy of the method.

### B. Force matching (FM)

To parametrize the FM potentials, the reference force on each coarse-grained bead $i$ is written in the following form:

$$\boldsymbol{f}_i^{\mathrm{ref}} = M_i \sum_{\alpha \in i} \frac{w_\alpha \boldsymbol{f}_\alpha}{m_\alpha}. \tag{II.4}$$

Here, $M_i$ is the mass of the CG bead $i$. The force on each CG bead is a weighted sum of the atomistic forces on all atoms belonging to this bead with mapping coefficients $w_\alpha$. The CG representation of the force is then determined by solving the following system of equations:

$$\boldsymbol{f}_{il}^{\mathrm{CG}}(g_1, \ldots, g_M) = \boldsymbol{f}_{il}^{\mathrm{ref}}, \quad i = 1, \ldots, N, \quad l = 1, \ldots, L. \tag{II.5}$$

The coefficients $g_1, \ldots, g_M$ are the coefficients of the chosen CG interaction potential or in other words the coefficients of the CG set of force-field basis functions. $N$ is the number of CG beads and $L$ is the number of simulation snapshots. In this work, $N = 1000$ and $L = 20$. Given that the CG force-field basis functions $f_{il}^{\mathrm{CG}}$ depend linearly on the parameters $g_1, \ldots, g_M$, equation (II.5) is a set of $N \times L$ overdetermined linear equations ($M < N \times L$).

In the case of pair interactions only, we choose cubic splines as force-field basis functions $f_{il}^{\mathrm{CG}}$ which depend linearly on the coefficients $g_1, \ldots, g_M$. Using the VOTCA implementation, described in detail in Ref. 4, a set of $K$ grid points leads to $M = 2K$ spline coefficients where $K$ of the coefficients are fixed due to constraints guaranteeing the continuity of the first derivatives. The set of equations (II.5) is then solved with a constrained least-squares solver. Afterwards, the CG interaction potentials are determined from the CG forces by numerical integration. Before integration, the tabulated two-body forces are multiplied by an analytic function of the form

$$f_{\mathrm{switch}}(r) = \cos\left(\frac{\pi}{2} \frac{r - r_{\mathrm{sm}}}{r_{\mathrm{cut}} - r_{\mathrm{sm}}}\right). \tag{II.6}$$

This is done for all distances greater than $r_{\mathrm{sm}} = 1.0$ to ensure a smooth decay to zero at the short range cutoff of $r_{\mathrm{cut}} = 1.2\,\mathrm{nm}$.

### C. Extension of the FM routine to three-body interactions

As described in the main text, we extend the two-body CG interactions with three-body interactions of the Stillinger-Weber (SW) form:

$$U^{\mathrm{SW}} = \sum_{i, j \neq i, k > j} f^{(3b)}(\theta_{ijk}) \exp\left(\frac{\gamma_{ij}\sigma_{ij}}{r_{ij} - a_{ij}\sigma_{ij}}\right) \exp\left(\frac{\gamma_{ik}\sigma_{ik}}{r_{ik} - a_{ik}\sigma_{ik}}\right). \tag{II.7}$$

In this notation, $i$ is the index of the central atom and $j$ and $k$ are the other two atom indices of a triplet of atoms with an angular interaction term $f^{(3b)}(\theta_{ijk})$. We do not limit ourselves to an analytic expression of $f^{(3b)}(\theta_{ijk})$ as in the original SW potential, but allow for a flexible angular dependence. In the following, we describe in detail the FM

parametrization of this flexible $U^{\mathrm{SW}}$ in the VOTCA framework. To obtain the set of equations (II.5), one has to calculate the force $\boldsymbol{f}_i^{\mathrm{SW}} = -\nabla_i U^{SW}$ coming from the SW interaction on each CG bead $i$, namely:

$$\begin{aligned}\boldsymbol{f}_i^{\mathrm{SW}} = &\left(\frac{\partial}{\partial\theta} f^{(3b)}(\theta)\right)(-\nabla_i\theta)\exp\left(\frac{\gamma_{ij}\sigma_{ij}}{r_{ij}-a_{ij}\sigma_{ij}}\right)\exp\left(\frac{\gamma_{ik}\sigma_{ik}}{r_{ik}-a_{ik}\sigma_{ik}}\right)\\ &+ f^{(3b)}\left[(-\nabla_i r_{ij})\left(-\frac{\gamma_{ij}\sigma_{ij}}{(r_{ij}-a_{ij}\sigma_{ij})^2}\right)\exp\left(\frac{\gamma_{ij}\sigma_{ij}}{r_{ij}-a_{ij}\sigma_{ij}}\right)\exp\left(\frac{\gamma_{ik}\sigma_{ik}}{r_{ik}-a_{ik}\sigma_{ik}}\right)\right.\\ &\left.+(-\nabla_i r_{ik})\left(-\frac{\gamma_{ik}\sigma_{ik}}{(r_{ik}-a_{ik}\sigma_{ik})^2}\right)\exp\left(\frac{\gamma_{ij}\sigma_{ij}}{r_{ij}-a_{ij}\sigma_{ij}}\right)\exp\left(\frac{\gamma_{ik}\sigma_{ik}}{r_{ik}-a_{ik}\sigma_{ik}}\right)\right],\end{aligned} \tag{II.8}$$

$$\begin{aligned}\boldsymbol{f}_j^{\mathrm{SW}} = &\left(\frac{\partial}{\partial\theta} f^{(3b)}(\theta)\right)(-\nabla_j\theta)\exp\left(\frac{\gamma_{ij}\sigma_{ij}}{r_{ij}-a_{ij}\sigma_{ij}}\right)\exp\left(\frac{\gamma_{ik}\sigma_{ik}}{r_{ik}-a_{ik}\sigma_{ik}}\right)\\ &+ f^{(3b)}\left[(-\nabla_j r_{ij})\left(-\frac{\gamma_{ij}\sigma_{ij}}{(r_{ij}-a_{ij}\sigma_{ij})^2}\right)\exp\left(\frac{\gamma_{ij}\sigma_{ij}}{r_{ij}-a_{ij}\sigma_{ij}}\right)\exp\left(\frac{\gamma_{ik}\sigma_{ik}}{r_{ik}-a_{ik}\sigma_{ik}}\right)\right],\end{aligned} \tag{II.9}$$

$$\begin{aligned}\boldsymbol{f}_k^{\mathrm{SW}} = &\left(\frac{\partial}{\partial\theta} f^{(3b)}(\theta)\right)(-\nabla_k\theta)\exp\left(\frac{\gamma_{ij}\sigma_{ij}}{r_{ij}-a_{ij}\sigma_{ij}}\right)\exp\left(\frac{\gamma_{ik}\sigma_{ik}}{r_{ik}-a_{ik}\sigma_{ik}}\right)\\ &+ f^{(3b)}\left[(-\nabla_k r_{ij})\left(-\frac{\gamma_{ik}\sigma_{ik}}{(r_{ik}-a_{ik}\sigma_{ik})^2}\right)\exp\left(\frac{\gamma_{ij}\sigma_{ij}}{r_{ij}-a_{ij}\sigma_{ij}}\right)\exp\left(\frac{\gamma_{ik}\sigma_{ik}}{r_{ik}-a_{ik}\sigma_{ik}}\right)\right].\end{aligned} \tag{II.10}$$

We represent $f^{(3b)}(\theta)$ with cubic splines with $g_1, \ldots, g_M$, $M = 2K$, spline coefficients (when using $K$ grid points) in the same way as the representation of the two-body force-field basis functions. The derivative $\frac{\partial}{\partial\theta} f^{(3b)}(\theta)$ is the analytical derivative of the cubic spline implementation, meaning the derivative is represented by a 2nd order polynomial. To obtain a linear set of equations, all terms in equations (II.8) to (II.10) except $f^{(3b)}(\theta)$ and $\frac{\partial}{\partial\theta} f^{(3b)}(\theta)$ are treated as prefactors. This allows to include equations (II.8) to (II.10) into the set of linear equations (II.5) which is solved by a constrained least-squares solver.

In contrast to the spline representation of the pair forces, the system of equations now includes, both, $f^{(3b)}(\theta)$ and $\frac{\partial}{\partial\theta} f^{(3b)}(\theta)$, due to application of the chain rule when calculating the derivative of $U^{\mathrm{SW}}$ (II.7). This implies that in this case the set of spline coefficients determines $f^{(3b)}(\theta)$ and $\frac{\partial}{\partial\theta} f^{(3b)}(\theta)$ simultaneously and no numerical integration is needed. Furthermore, the remaining coefficients of the SW potential (II.7), $a_{ij}$, $a_{ik}$, $\sigma_{ij}$, $\sigma_{ik}$, $\gamma_{ij}$, and $\gamma_{ik}$, have to be set beforehand. In the case of only one CG bead type, as in this work, this reduces to: $a_{ij} = a_{ik} = a$, $\sigma_{ij} = \sigma_{ik} = \sigma$, and $\gamma_{ij} = \gamma_{ik} = \gamma$ leaving 3 free parameters to be fixed. In fact, $a$ is the three-body short-range cutoff radius and the two exponential terms $\exp\left(\frac{\gamma\sigma}{r-a\sigma}\right)$ of the SW potential ensure a smooth switching on of the three-body interaction whenever a triplet of atoms is within the cutoff radius $a$. Setting $\sigma = 1$, the remaining parameter $\gamma$ fixes the "steepness" of this switching on. In practice, $a$ and $\gamma$ have to be set by physical intuition. A reasonable parameter choice is such that the SW potential is fully switched on in the first coordination shell. In the case of SPC/E water we refer to the values of Ref. 15 ($a = 0.37$ nm and $\gamma = 0.12$ nm). In the case of methanol, we screened different values of $a$ and $\gamma$ such that $U^{\mathrm{SW}}$ is switched on in the first coordination shell. We obtain the best results for $a = 0.45$ nm and $\gamma = 0.08$ nm. However, the qualitative results of this work do not depend on the exact values of $a$ and $\gamma$ when chosen in a way that $U^{\mathrm{SW}}$ is switched on in the first and switched off within the second coordination shell.

## III. POTENTIAL OF MEAN FORCE

The two-body PMFs is evaluated as

$$U_{\mathrm{PMF}}(r) = \int_{\infty}^{r} F_r(r')\,\mathrm{d}r' \tag{III.1}$$

where $F_r(r)$ is the radial component of the total force on a CG bead averaged over all pairs of CG beads with distance $r$. $F_r(r)$ is evaluated in the CG simulation run with the respective CG interaction potential or in the atomistic simulation by employing the CG mapping (II.1). Having different force contributions, $F_r(r)$ and, thus, the PMF can be evaluated for each force contribution individually by performing a simulation rerun with switching on and off each contribution of the total CG interaction potential. By doing so, we are able to evaluate the contribution to the total two-body PMF coming from the two-body and three-body basis functions.

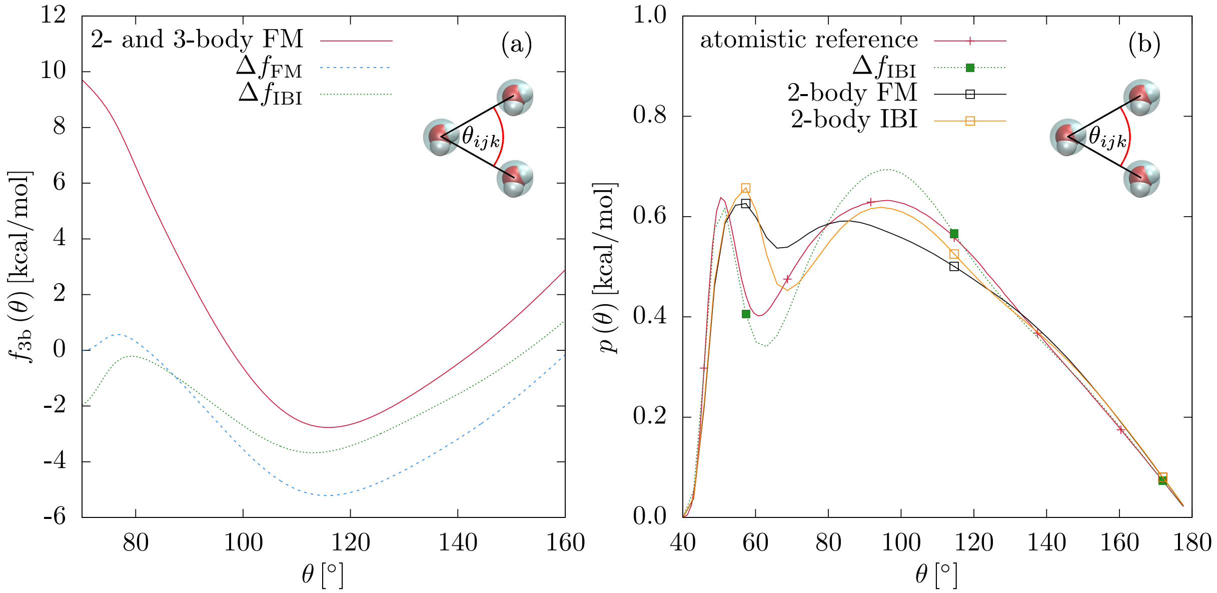


FIG. 1. (a) $f^{(3b)}(\theta_{ijk})$ prefactor in the SW three-body potential (II.7). (b) Angular distribution functions of coarse-grained SPC/E water. The different CG parametrizations refer to: two-body force matching (2-body FM), two-body structural matching (2-body IBI), concurrent force-matching with tabulated pair potentials and the short-range three-body SW potential (2- and 3-body FM), three-body FM using the residual force of the two-body FM potential ($\Delta f_{\mathrm{FM}}$), and three-body FM using the residual force of the two-body IBI potential ($\Delta f_{\mathrm{IBI}}$).

## IV. ENTHALPY OF VAPORIZATION

In the main text, we compare total pressures and enthalpies of vaporization of the atomistic and the CG simulations. All pressures refer to the virial pressures, including all two-body, three-body and electrostatic long-range interactions.[16] The molar enthalpies of vaporization $\Delta H$ or, in other words, the enthalpy differences between the gas phase and the liquid phase are calculated according to the formulation in Refs. 10 and 17:

$$\Delta H = H_{\mathrm{gas}} - H_{\mathrm{liq}} = \langle E_{\mathrm{int,gas}} + p_{\mathrm{gas}} V_{\mathrm{gas}} \rangle - \langle E_{\mathrm{int,liq}} + p_{\mathrm{liq}} V_{\mathrm{liq}} \rangle = \langle E_{\mathrm{pot,gas}} \rangle + RT - \langle E_{\mathrm{pot,liq}} + p_{\mathrm{liq}} V_{\mathrm{liq}} \rangle \,. \tag{IV.1}$$

The internal energies, $E_{\mathrm{int,gas}} = E_{\mathrm{pot,gas}} + E_{\mathrm{kin,gas}}$ and $E_{\mathrm{int,liq}} = E_{\mathrm{pot,liq}} + E_{\mathrm{kin,liq}}$, refer to the total internal energies of the liquid phase and the gas phase, normalized to one molecule. As we consider the liquid state and the gas state at the same temperature ($T = 300\,\mathrm{K}$), the average kinetic energies $\langle E_{\mathrm{kin,gas}} \rangle$ and $\langle E_{\mathrm{kin,liq}} \rangle$ cancel out and only the difference of the average total potential (cohesive) energies is relevant: $\langle E_{\mathrm{pot,gas}} \rangle - \langle E_{\mathrm{pot,liq}} \rangle$ (see equation (IV.1)). In principle, both, consist of inter- and intra-molecular contributions $E_{\mathrm{inter}}$ and $E_{\mathrm{intra}}$. In case of the all-atom simulations, we determine $E_{\mathrm{pot,gas}}$ with gas phase simulations at $T = 300\,\mathrm{K}$ with one single molecule in a simulation box of $L_{box} = 10\,\mathrm{nm}$ (see Ref. 10). In doing so, we assume that there is no intra-molecular contribution to the gas phase potential energy: $E_{\mathrm{pot,gas}} \simeq E_{\mathrm{intra,gas}}$. In case of a single bead CG representation as used in this work, there is no intra-molecular potential energy in the gas phase at all and the total potential energy of the gas phase is assumed to be $E_{\mathrm{pot,gas}} \simeq 0$. This means, we assume the CG gas to be an ideal gas (following the argumentation in Ref. 17) with a total enthalpy of $H_{\mathrm{gas}} = 2.5\,RT$ with $1.5\,RT$ attributed to the (canceled out) kinetic energy $E_{\mathrm{kin,gas}}$ and $1.0\,RT$ attributed to $\langle p_{\mathrm{gas}} V_{\mathrm{gas}} = RT \rangle$ (equation of state of an ideal gas). In the case of the all-atom NVT MD simulations, the average liquid pressure is basically equal to zero: $p_{\mathrm{liq}} = 1\,\mathrm{bar} \simeq 0$. Therefore, the term $\langle p_{\mathrm{liq}} V_{\mathrm{liq}} \rangle$ can be neglected when evaluating equation (III.1). In case of the CG NVT MD simulations (which are conducted at the atomistic density), we have to explicitly evaluate $\langle p_{\mathrm{liq}} V_{\mathrm{liq}} \rangle$.

## V. STRUCTURE AND TWO-BODY PMF OF LIQUID WATER

In the following, we show CG potentials, distribution functions and potentials of means force (PMFs) of liquid SCP/E water that are not shown in the main text.

In Fig. 1(a) we show the tabulated angular part of the short-range three-body SW potential (II.7), $f^{(3b)}(\theta_{ijk})$, for all different CG parametrizations of SPC/E water. One can clearly see that the parametrizations of the residual forces $\Delta\boldsymbol{f}_i$, i.e., after subtracting the two-body force from the total force on each CG bead, lead to a shift of $f(\theta)$. This holds for both the two-body FM and IBI forces. In Fig. 1(b), the angular distributions of all CG water potentials are depicted that are not shown in Fig.4(b) of the main text. One can clearly see that the two CG potentials with only pair potentials (2-body FM and 2-body IBI) have angular distributions fairly different from the atomistic reference.

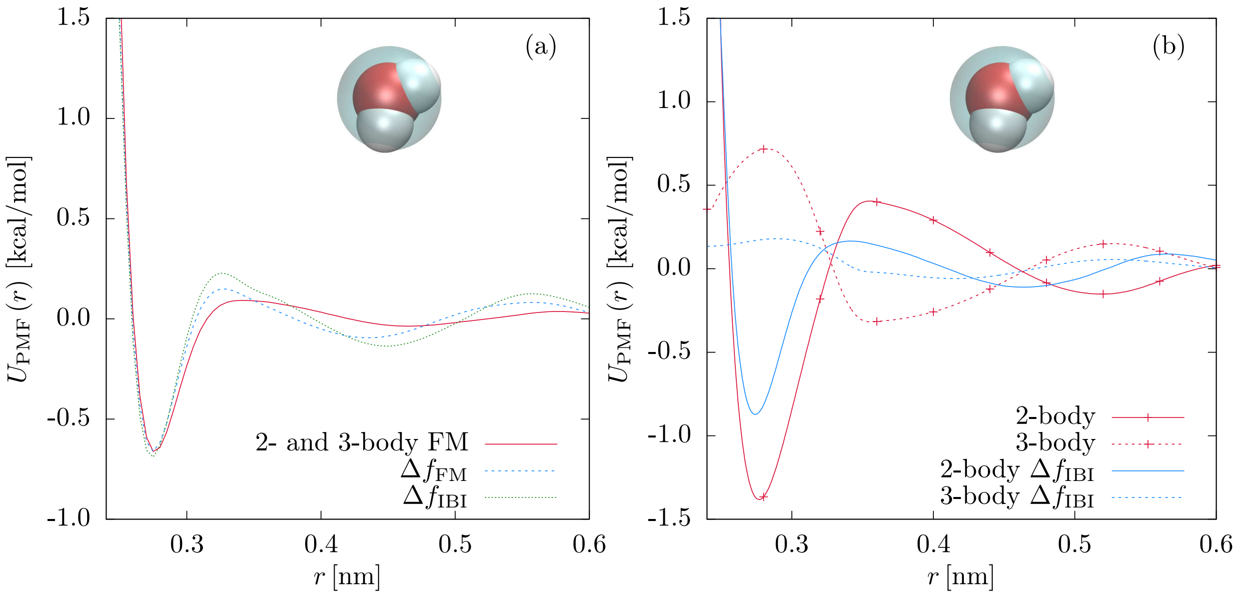


FIG. 2. CG two-body potentials of mean force (PMF) for liquid SPC/E water: (a) The total PMFs for three different parametrizations: concurrent force-matching with tabulated pair potentials and the short-range three-body SW potential (2- and 3-body FM), three-body FM using the residual force of the two-body FM potential ($\Delta f_{\mathrm{FM}}$), and three-body FM using the residual force of the two-body IBI potential ($\Delta f_{\mathrm{IBI}}$).(b) The splitting of the total PMF into 2-body and 3-body contributions for the following CG potentials: 2- and 3-body FM (curve 1 and 2), $\Delta f_{\mathrm{IBI}}$ (curve 3 and 4).

In Fig. 2(a), we show the total two-body PMF for all CG potentials of SPC/E water including short-range three-body interactions. The first curve refers to the concurrent parametrization of two- and three-body interactions. The second and the third curve refer to the parametrizations according to the residual forces ($\Delta f_{\mathrm{FM}}$ and $\Delta f_{\mathrm{IBI}}$). This information complements Fig.2(a) of the main text. In Fig. 2(a), we show the splitting of the total two-body PMF into the two-body and three-body contributions for CG SPC/E water. Here, the splitting of the parametrization according to the residual force of the structure matching scheme ($\Delta f_{\mathrm{IBI}}$) is compared to the concurrent two-body and three-body parametrization (2-body and 3-body FM). This complements Fig.3(a) of the main text. It can be clearly seen that three-body contribution to the two-body PMF is significantly reduced also for the $\Delta f_{\mathrm{IBI}}$ parametrization.

## VI. STRUCTURE AND TWO-BODY PMF OF LIQUID METHANOL

In the following, we show CG potentials, distribution functions and potentials of means force (PMFs) of liquid methanol that are not shown in the main text.

In Fig. 3(a), we show all different pair potentials for liquid methanol. The first two curves refer to the two-body parametrizations (2-body IBI and 2-body FM). In the case of methanol, these two potentials are practically identical, in contrast to SPC/E water (see Fig. 1(a) of the main text). This, again, shows that projection on only two-body basis functions is a significantly better representation of the CG PMF for methanol than for SPC/E water. The third curve shows the two-body part of the concurrent FM two- and three-body parametrization (2- and 3-body FM). As in the case of water (Fig. 1(a) of the main text), adding a short-ranged three-body term leads to a significantly more attractive two-body interaction. In Fig. 3(b), we show the radial distribution functions for all different CG force-fields of methanol. Basically, all parametrizations lead to nearly identical results. (The two-body IBI curve is omitted as it is practically identical to the atomistic reference curve due to construction.) This is in contrast to the observation for the CG SPC/e water models (see Fig.1(b) of the main text). The parametrization of the three-body interactions according to the residual force ($\Delta f_{\mathrm{FM}}$ and $\Delta f_{\mathrm{IBI}}$) show a slight decrease of the height of first- and increase of the

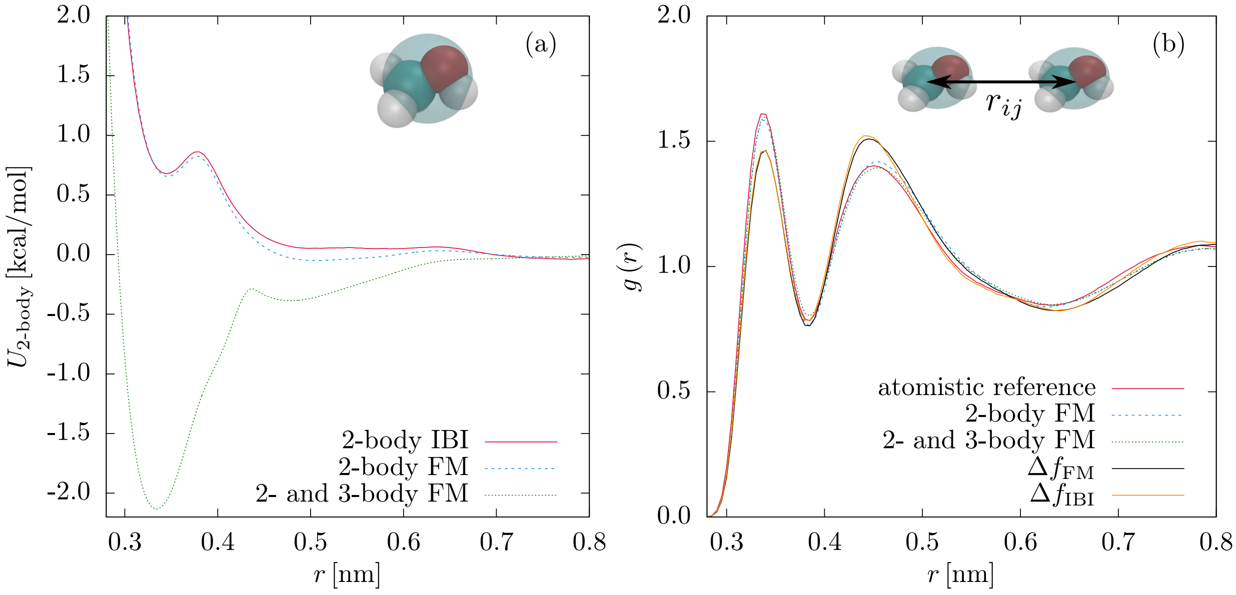


FIG. 3. (a) Pair potentials and (b) radial distribution functions of coarse-grained methanol. Three following parametrizations are shown: structural matching (2-body IBI), force matching using (tabulated) pair potentials only (2-body FM), force-matching with tabulated pair potentials and the short-range three-body SW potential (2- and 3-body FM), three-body FM using the residual force of the two-body FM potential ($\Delta f_{\mathrm{FM}}$), and three-body FM using the residual force of the two-body IBI potential ($\Delta f_{\mathrm{IBI}}$). The CG IBI radial distribution function perfectly matches the atomistic reference curve by construction.

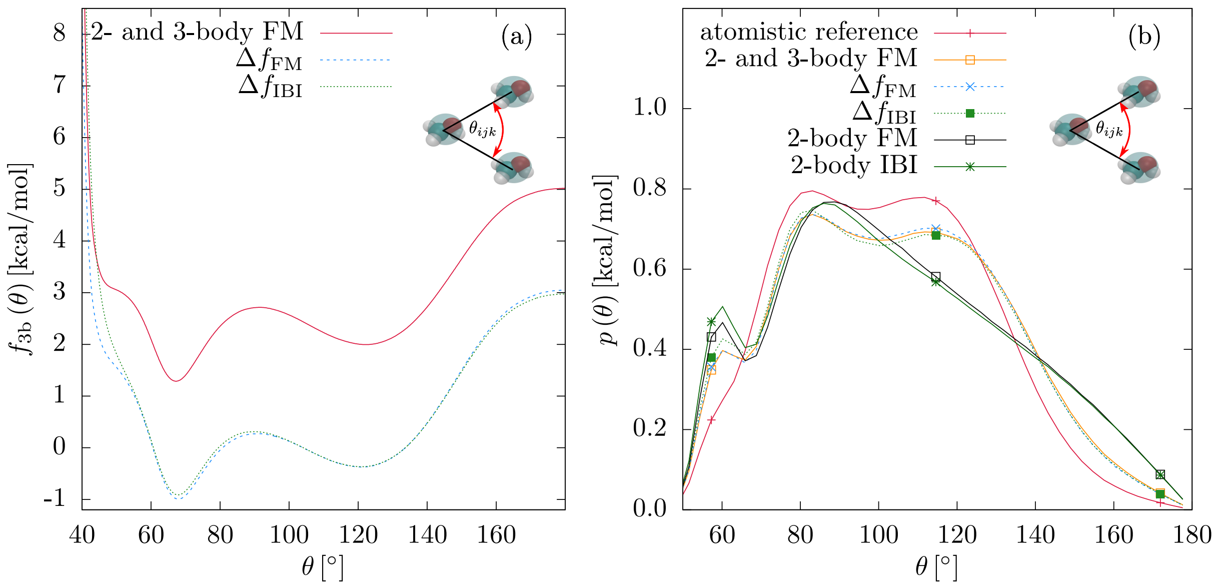


FIG. 4. (a) $f^{(3b)}(\theta_{ijk})$ prefactor of the SW three-body potential (II.7). (b) Angular distribution functions of coarse-grained methanol. The different CG parametrizations refer to: two-body force matching (2-body FM), two-body structural matching (2-body IBI), concurrent force-matching with tabulated pair potentials and the short-range three-body SW potential (2- and 3-body FM), three-body FM using the residual force of the two-body FM potential ($\Delta f_{\mathrm{FM}}$), and three-body FM using the residual force of the two-body IBI potential ($\Delta f_{\mathrm{IBI}}$).

second-neighbor peak compared to the atomistic reference curve. This is attributed to the short-range repulsion of the additional three-body SW potential.

In Fig. 4(a) we show the tabulated angular part of the short-range three-body SW potential (II.7), $f^{(3b)}(\theta_{ijk})$, for all different CG parametrizations of liquid methanol. One can clearly see that the parametrizations according to the residual forces $\Delta \boldsymbol{f}_i$, i.e., after subtracting the two-body force from the total force on each CG bead $i$: $\Delta \boldsymbol{f}_i = \boldsymbol{f}_i^{\mathrm{ref}} - \boldsymbol{f}_i^{\text{2-body}}$ mainly lead to a shift of $f(\theta)$. This holds for, both, the two-body FM, as well as, the two-body IBI

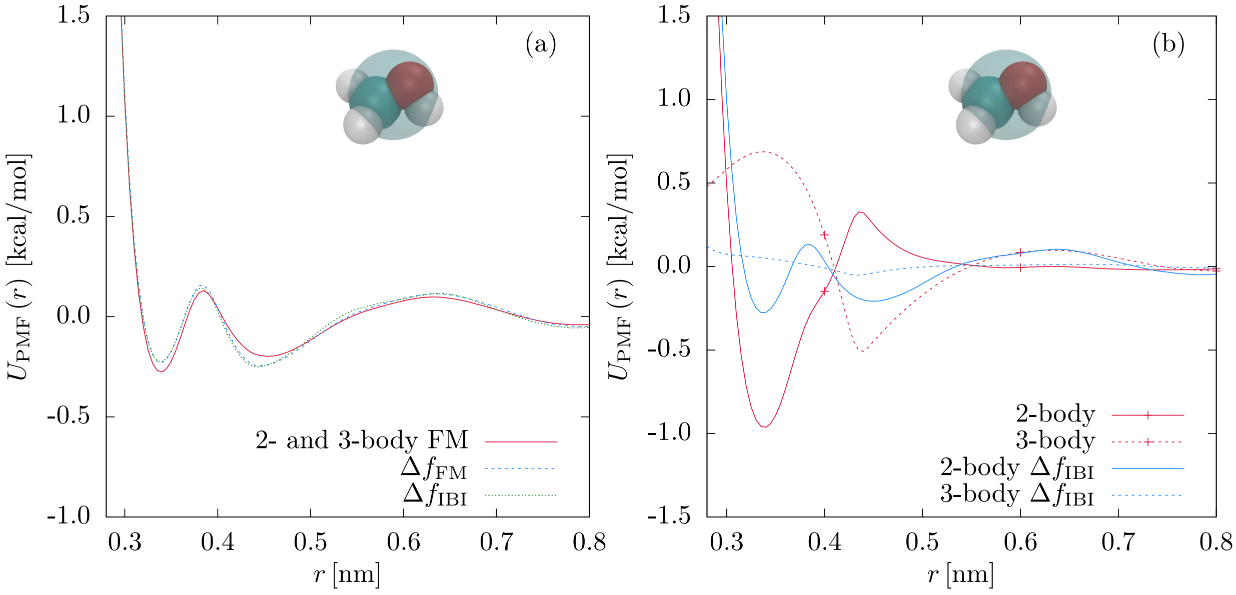


FIG. 5. CG two-body potentials of mean force (PMF) for liquid SPC/E water: (a) The total PMFs for three different parametrizations: concurrent force-matching with tabulated pair potentials and the short-range three-body SW potential (2- and 3-body FM), three-body FM using the residual force of the two-body FM potential ($\Delta f_{\mathrm{FM}}$), and three-body FM using the residual force of the two-body IBI potential ($\Delta f_{\mathrm{IBI}}$).(b) The splitting of the total PMF into 2-body and 3-body contributions for the following CG potentials: 2- and 3-body FM (curve 1 and 2), $\Delta f_{\mathrm{IBI}}$ (curve 3 and 4).

force. For methanol, the two curves ($\Delta f_{\mathrm{FM}}$ and $\Delta f_{\mathrm{IBI}}$) are practically identical. This is due to the nearly identical FM and IBI pair potentials (see Fig. 3)(a). In Fig. 1(b), the angular distributions of all CG methanol potentials are shown. One can clearly see that all CG potentials including short-range three-body terms (2- and 3-body FM, $\Delta f_{\mathrm{FM}}$, and $Delta f_{\mathrm{IBI}}$) show a significantly better agreement to the atomistic reference distribution than the CG potential only containing pair interactions (2-body FM and 2-body IBI).

In Fig. 5(a), we show the total two-body PMF for all CG potentials of liquid methanol including short-range three-body interactions. The first curve refers to the concurrent parametrization of two- and three-body interactions. The second and the third curve refer to the parametrizations according to the residual forces ($\Delta f_{\mathrm{FM}}$ and $\Delta f_{\mathrm{IBI}}$). This information complements Fig.2(b) of the main text. In Fig. 5(a), we show the splitting of the total two-body PMF into the two-body and three-body contributions for CG methanol. Here, the splitting of the parametrization according to the residual force of the structure matching scheme ($\Delta f_{\mathrm{IBI}}$) is compared to the concurrent two-body and three-body parametrization (2-body and 3-body FM). This complements Fig.3(b) of the main text. It can be clearly seen that three-body contribution to the two-body PMF is significantly reduced also for the $\Delta f_{\mathrm{IBI}}$ parametrization.

## REFERENCES


[1] H. J. C. Berendsen, J. R. Grigera, and T. P. Straatsma, Journal of Physical Chemistry **91**, 6269 (1987).
[2] W. L. Jorgensen and J. Tirado-Rives, Journal of the American Chemical Society **110**, 1657 (1988).
[3] W. L. Jorgensen, D. S. Maxwell, and J. Tirado-Rives, Journal of the American Chemical Society **118**, 11225 (1996).
[4] V. Rühle, C. Junghans, A. Lukyanov, K. Kremer, and D. Andrienko, Journal of Chemical Theory and Computation **5**, 3211 (2009).
[5] M. J. Abraham, T. Murtola, R. Schulz, S. Páll, J. C. Smith, B. Hess, and E. Lindahl, SoftwareX **1-2**, 19 (2015).
[6] W. F. Van Gunsteren and H. J. C. Berendsen, Molecular Simulation **1**, 173 (1988).
[7] H. J. Berendsen, J. v. Postma, W. F. van Gunsteren, A. DiNola, and J. R. Haak, The Journal of chemical physics **81**, 3684 (1984).
[8] U. Essmann, L. Perera, M. L. Berkowitz, T. Darden, H. Lee, and L. G. Pedersen, The Journal of Chemical Physics **103**, 8577 (1995).
[9] J. L. F. Abascal and C. Vega, The Journal of Chemical Physics **123**, 234505 (2005).
[10] C. Caleman, P. J. van Maaren, M. Hong, J. S. Hub, L. T. Costa, and D. van der Spoel, Journal of Chemical Theory and Computation **8**, 61 (2012).
[11] S. Plimton, Journal of Computational Physics **117**, 1 (1995).
[12] S. Nosé, Molecular Physics **52**, 255 (1984).
[13] W. G. Hoover, Physical Review A **31**, 1695 (1985).
[14] W. Shinoda, M. Shiga, and M. Mikami, Physical Review B **69** (2004).
[15] L. Larini, L. Lu, and G. A. Voth, The Journal of Chemical Physics **132**, 164107 (2010).
[16] A. P. Thompson, S. J. Plimpton, and W. Mattson, The Journal of Chemical Physics **131**, 154107 (2009).

[17] J. Lu, Y. Qiu, R. Baron, and V. Molinero, Journal of Chemical Theory and Computation **10**, 4104 (2014).
